# Supplementary material for: Security Apps under the Looking Glass: An Empirical Analysis of Android Security Apps
Source: arXiv:2007.03905 source file (2020-07-08)
Supplement: Supplementary file 1 [file AppendixA.tex]

\section{Appendix}
\label{sec:Appendix}

\subsection{K-Means Clustering Results}
Table~\ref{tab:AppA} shows list of apps in each of two clusters.

\begin{table}[]
\scriptsize
\caption{List of Antivirus Apps in Both Clusters}

\label{tab:AppA}
\begin{tabular}{|l|l|}
\hline
\textbf{Cluster : Virus Detector/ Scanner} & \textbf{Cluster 2: Virus Cleaning}             \\ \hline
com.cleanmaster.security                   & com.cleanmaster.mguard                         \\ \hline
com.samsung.android.lool                   & com.dianxinos.optimizer.duplay                 \\ \hline
com.qihoo.security                         & com.lionmobi.powerclean                        \\ \hline
com.antivirus                              & com.apps.go.clean.boost.master                 \\ \hline
com.psafe.msuite                           & com.cmcm.lite                                  \\ \hline
com.avast.android.mobilesecurity           & com.qihoo.security.lite                        \\ \hline
com.drweb                                  & com.ehawk.antivirus.applock.wifi               \\ \hline
com.lookout                                & com.avg.cleaner                                \\ \hline
com.kms.free                               & com.piriform.ccleaner                          \\ \hline
com.zrgiu.antivirus                        & com.oneapp.max.cleaner.booster                 \\ \hline
com.lm.powersecurity                       & com.hyperspeed.rocketclean.pro                 \\ \hline
com.symantec.mobilesecurity                & com.oneapp.max.security.pro                    \\ \hline
com.jb.security                            & com.avast.android.cleaner                      \\ \hline
com.wsandroid.suite                        & com.rocket.tools.clean.antivirus.master        \\ \hline
com.drweb.pro                              & com.hyperspeed.rocketclean                     \\ \hline
com.eset.ems2.gp                           & phone.cleaner.speed.booster.                   \\ \hline
com.bugsecapps.droidbughaunterfree         & cache.clean.android.master                     \\ \hline
imoblife.toolbox.full                      & smart.booster.antivirus                        \\ \hline
com.avira.android                          & com.apps.power.super.clean.security.master     \\ \hline
com.trustlook.antivirus                    & com.ant.cleaner                                \\ \hline
com.duapps.antivirus                       & antivirus.anti.virus.cleaner.security.booster  \\ \hline
com.nqmobile.antivirus20                   & com.iobit.amccleaner.booster                   \\ \hline
com.trendmicro.freetmms.gmobi              & com.falcon.antivirus                           \\ \hline
com.guardian.security.pri                  & cleaner.antivirussecurity.booster              \\ \hline
com.s.antivirus                            & com.virus.removal.for.android                  \\ \hline
com.fluerapps.antivirus2017freepremium     & com.immunesmart.security.junkcleaner.          \\ \hline
com.vainfoantivirus2019tomar               & cacheremover.power.booster.cleanram.           \\ \hline
com.mans.antivirus.security                & antivirus.memory.master.cooler.fast.speed.free \\ \hline
com.bettertomorrowapps.camerablockfree     & antivirus.virusremoval.security.phone          \\ \hline
com.mobincube.android.sc\_GM86R            & com.lstudio.freeantivirus                      \\ \hline
com.sophos.appprotectionmonitor            & frouza.antivirus.security.cleaner.             \\ \hline
com.androhelm.antivirus.premium            & booster.batterysaver.applock                   \\ \hline
smart.anti.virus.phone                     & com.asteamsecurityphonelab.                    \\ \hline
at.ncn.antiviruspro2016                    & mobileantivirus.applock                        \\ \hline
com.omelettestudios.TrackingAlert          & com.msysoft.viruscleaner.security              \\ \hline
com.hidden.apps.detector                   & freeantivirus.free.antivirus                   \\ \hline
com.ashampoo.rottensyschecker              & com.galaxy.powerclean2020                      \\ \hline
com.androhelm.antivirus.free               & com.ayogamez.antiviruscleaner.forandroid       \\ \hline
com.eset.securedialer                      & com.free.antivirus.virusscan.cleaner           \\ \hline
com.nettoyage.mobile                       & com.jixic.antivirus.for.android.phone          \\ \hline
com.looptoop.applocker2017                 &                                                \\ \hline
com.wsandroid.suite.tmobile                &                                                \\ \hline
com.bullguard.mobile.mobilesecurity        &                                                \\ \hline
com.zemana.msecurity                       &                                                \\ \hline
com.drweb.mcc                              &                                                \\ \hline
com.aegislab.sd3prj.premium                &                                                \\ \hline
com.bitdefender.centralmgmt                &                                                \\ \hline
com.max.gamerantivirus                     &                                                \\ \hline
com.lacoon.security.fox                    &                                                \\ \hline
erfanrouhani.antispy                       &                                                \\ \hline
antivirus.maka.scannner.security           &                                                \\ \hline
com.virusremove.antiviruss.antimwaerihr    &                                                \\ \hline
com.max.maxantivirus                       &                                                \\ \hline
com.applock.antiviruss.mobilesecurity      &                                                \\ \hline
at.ncn.antiviruspro                        &                                                \\ \hline
at.ncn.virusremove2018                     &                                                \\ \hline
com.theantivirus.cleanerandbooster         &                                                \\ \hline
com.fluerapps.antivirus2019freepremium     &                                                \\ \hline
com.andromo.dev746210.app822980            &                                                \\ \hline
mobileshield.antivirus                     &                                                \\ \hline
com.appsplan1.freespywareremovalinfo       &                                                \\ \hline
amigoskey.antivirus                        &                                                \\ \hline
com.securitydefend.totalvirusdefenderfull  &                                                \\ \hline
com.amantechnoapps.antivirusfree2019       &                                                \\ \hline
\end{tabular}
\end{table}

% Please add the following required packages to your document preamble:
% \usepackage{longtable}
% Note: It may be necessary to compile the document several times to get a multi-page table to line up properly
\onecolumn
{\scriptsize
\begin{longtable}{|l|l|l|}

\caption{}
\label{tab:my-table}\\

\hline
\textbf{Permissions} & \textbf{Category} & \textbf{Number of Apps} \\ \hline
\endfirsthead
\endhead

INTERNET & Normal & 98 \\ \hline
ACCESS\_NETWORK\_STATE & Normal & 97 \\ \hline
WAKE\_LOCK & Normal & 88 \\ \hline
WRITE\_EXTERNAL\_STORAGE & Dangerous & 85 \\ \hline
RECEIVE\_BOOT\_COMPLETED & Normal & 83 \\ \hline
ACCESS\_WIFI\_STATE & Normal & 78 \\ \hline
READ\_EXTERNAL\_STORAGE & Dangerous & 77 \\ \hline
RECEIVE & Normal & 72 \\ \hline
READ\_PHONE\_STATE & Dangerous & 68 \\ \hline
VIBRATE & Normal & 67 \\ \hline
GET\_TASKS & Normal & 65 \\ \hline
KILL\_BACKGROUND\_PROCESSES & Normal & 62 \\ \hline
SYSTEM\_ALERT\_WINDOW & Dangerous & 61 \\ \hline
GET\_PACKAGE\_SIZE & Normal & 57 \\ \hline
GET\_ACCOUNTS & Dangerous & 53 \\ \hline
CAMERA & Dangerous & 52 \\ \hline
CHANGE\_WIFI\_STATE & Normal & 52 \\ \hline
CLEAR\_APP\_CACHE & Dangerous & 52 \\ \hline
WRITE\_SETTINGS & Normal & 49 \\ \hline
BILLING & Normal & 46 \\ \hline
BIND\_GET\_INSTALL\_REFERRER\_SERVICE & Normal & 46 \\ \hline
C2D\_MESSAGE & Normal & 46 \\ \hline
INSTALL\_SHORTCUT & Normal & 45 \\ \hline
READ\_HISTORY\_BOOKMARKS & Normal & 45 \\ \hline
ACCESS\_FINE\_LOCATION & Dangerous & 44 \\ \hline
ACCESS\_COARSE\_LOCATION & Dangerous & 39 \\ \hline
WRITE\_HISTORY\_BOOKMARKS & Normal & 39 \\ \hline
CHANGE\_NETWORK\_STATE & Normal & 37 \\ \hline
EXPAND\_STATUS\_BAR & Normal & 32 \\ \hline
UNINSTALL\_SHORTCUT & Normal & 32 \\ \hline
READ\_SETTINGS & Normal & 31 \\ \hline
READ\_CONTACTS & Dangerous & 30 \\ \hline
BLUETOOTH & Normal & 29 \\ \hline
READ\_LOGS & Normal & 28 \\ \hline
BLUETOOTH\_ADMIN & Normal & 26 \\ \hline
CALL\_PHONE & Dangerous & 26 \\ \hline
MANAGE\_ACCOUNTS & Normal & 26 \\ \hline
RESTART\_PACKAGES & Normal & 25 \\ \hline
MODIFY\_AUDIO\_SETTINGS & Normal & 24 \\ \hline
DISABLE\_KEYGUARD & Normal & 20 \\ \hline
FLASHLIGHT & Normal & 20 \\ \hline
READ\_SYNC\_SETTINGS & Normal & 20 \\ \hline
USE\_FINGERPRINT & Normal & 20 \\ \hline
WRITE\_SYNC\_SETTINGS & Normal & 20 \\ \hline
READ\_GSERVICES & Normal & 19 \\ \hline
WRITE\_CONTACTS & Dangerous & 19 \\ \hline
AUTHENTICATE\_ACCOUNTS & Normal & 17 \\ \hline
USE\_CREDENTIALS & Normal & 17 \\ \hline
SET\_ALARM & Normal & 16 \\ \hline
ACCESS\_NOTIFICATION\_POLICY & Normal & 15 \\ \hline
ACTIVITY\_RECOGNITION & Normal & 12 \\ \hline
WRITE\_USE\_APP\_FEATURE\_SURVEY & Normal & 12 \\ \hline
FOREGROUND\_SERVICE & Normal & 11 \\ \hline
READ & Normal & 11 \\ \hline
BROADCAST\_BADGE & Normal & 10 \\ \hline
UPDATE\_SHORTCUT & Normal & 10 \\ \hline
WRITE & Normal & 10 \\ \hline
BROADCAST\_STICKY & Normal & 9 \\ \hline
RECORD\_AUDIO & Dangerous & 9 \\ \hline
REORDER\_TASKS & Normal & 9 \\ \hline
REQUEST\_DELETE\_PACKAGES & Normal & 8 \\ \hline
UPDATE\_COUNT & Normal & 8 \\ \hline
WRITE\_INTERNAL\_STORAGE & Normal & 8 \\ \hline
WRITE\_SECURE\_SETTINGS & Normal & 8 \\ \hline
SYSTEM\_OVERLAY\_WINDOW & Normal & 7 \\ \hline
WRITE\_LOGS & Normal & 7 \\ \hline
CACHE\_PERMISSION & Normal & 6 \\ \hline
FRAMEWORK\_SECURITY & Normal & 6 \\ \hline
GOLDENEYE\_SECURITY & Normal & 6 \\ \hline
IDS\_PERMISSION & Normal & 6 \\ \hline
READ\_SYNC\_STATS & Normal & 6 \\ \hline
REQUEST\_IGNORE\_BATTERY\_OPTIMIZATIONS & Normal & 6 \\ \hline
TEMPORARY\_DISABLE & Normal & 6 \\ \hline
WRITE\_CALENDAR & Dangerous & 6 \\ \hline
CHANGE\_WIFI\_MULTICAST\_STATE & Normal & 5 \\ \hline
PERMISSION & Normal & 4 \\ \hline
PowerBoost & Normal & 4 \\ \hline
READ\_CALENDAR & Dangerous & 4 \\ \hline
SET\_WALLPAPER & Normal & 4 \\ \hline
ACCESS\_SUPERUSER & Normal & 3 \\ \hline
CHECK\_LICENSE & Normal & 3 \\ \hline
READ\_SMS & Dangerous & 3 \\ \hline
RECEIVE\_SMS & Dangerous & 3 \\ \hline
SEND\_SMS & Dangerous & 3 \\ \hline
STATE\_INFORMER\_SERVICE & Normal & 3 \\ \hline
WRITE\_SMS & Dangerous & 3 \\ \hline
ACCESS\_COARSE\_UPDATES & Normal & 2 \\ \hline
ACCESS\_DOWNLOAD\_MANAGER & Normal & 2 \\ \hline
ACCESS\_LOCATION\_EXTRA\_COMMANDS & Normal & 2 \\ \hline
AIRPLANE\_MODE & Normal & 2 \\ \hline
APPLICATION\_INTERFACE & Normal & 2 \\ \hline
BATTERY\_CHANGED\_ACTION & Normal & 2 \\ \hline
DEVICE\_INTERFACE & Normal & 2 \\ \hline
DOWNLOAD\_WITHOUT\_NOTIFICATION & Normal & 2 \\ \hline
FILESYSTEM\_INTERFACE & Normal & 2 \\ \hline
GPS\_ENABLED\_CHANGE & Normal & 2 \\ \hline
INTERPROCESS\_INTERFACE & Normal & 2 \\ \hline
PROCESS\_OUTGOING\_CALLS & Dangerous & 2 \\ \hline
RAISED\_THREAD\_PRIORITY & Normal & 2 \\ \hline
READ\_CALL\_LOG & Dangerous & 2 \\ \hline
READ\_SECURE\_SETTINGS & Normal & 2 \\ \hline
RECEIVE\_ADM\_MESSAGE & Normal & 2 \\ \hline
SECURITY\_INTERFACE & Normal & 2 \\ \hline
WRITE\_CALL\_LOG & Dangerous & 2 \\ \hline
ACCESS\_ALL\_DOWNLOADS & Normal & 1 \\ \hline
ACCESS\_DOWNLOAD\_MANAGER\_ADVANCED & Normal & 1 \\ \hline
ACCESS\_FINGERPRINT\_MANAGER & Normal & 1 \\ \hline
ACCESS\_LAUNCHER\_DATA & Normal & 1 \\ \hline
ANTI\_VIRUS & Normal & 1 \\ \hline
BADGE\_COUNT\_READ & Normal & 1 \\ \hline
BADGE\_COUNT\_WRITE & Normal & 1 \\ \hline
BIND\_DEVICE\_SECURITY & Normal & 1 \\ \hline
BROADCAST & Normal & 1 \\ \hline
CHANGE\_BADGE & Normal & 1 \\ \hline
COM\_WSSNPS & Normal & 1 \\ \hline
DATAMAP\_PERMISSION & Normal & 1 \\ \hline
DIAGMON & Normal & 1 \\ \hline
FIRST\_LAUNCH & Normal & 1 \\ \hline
FLASHLIGHTlj & Normal & 1 \\ \hline
INVOKE & Normal & 1 \\ \hline
INVOKE\_INTERNAL\_HANDLER & Normal & 1 \\ \hline
INVOKE\_WIPE\_FEATURES & Normal & 1 \\ \hline
MAPS\_RECEIVE & Normal & 1 \\ \hline
MEDIA\_CONTENT\_CONTROL & Normal & 1 \\ \hline
NET\_RAW & Normal & 1 \\ \hline
NFC & Normal & 1 \\ \hline
NOTIFICATION\_FILTER\_PERMISSION & Normal & 1 \\ \hline
PAYMENT\_BROADCAST\_PERMISSION & Normal & 1 \\ \hline
PROVIDER & Normal & 1 \\ \hline
PROVIDER\_INSERT\_BADGE & Normal & 1 \\ \hline
READ\_ALARM & Normal & 1 \\ \hline
READ\_APP\_BADGE & Normal & 1 \\ \hline
READ\_BOOST\_DATA & Normal & 1 \\ \hline
READ\_DMF\_DATA & Normal & 1 \\ \hline
READ\_MS\_DATA & Normal & 1 \\ \hline
READ\_PLAY\_MUSIC & Normal & 1 \\ \hline
READ\_PROFILE & Normal & 1 \\ \hline
READ\_SEC\_COMMON\_POLICY & Normal & 1 \\ \hline
READ\_SM\_DATA & Normal & 1 \\ \hline
RECEIVE\_USER\_PRESENT & Normal & 1 \\ \hline
RECEIVE\_WAP\_PUSH & Dangerous & 1 \\ \hline
REGISTER\_ACCOUNT & Normal & 1 \\ \hline
REMOTE\_LOCK\_SERVICE & Normal & 1 \\ \hline
SCAN & Normal & 1 \\ \hline
SEND & Normal & 1 \\ \hline
SEND\_COMMAND & Normal & 1 \\ \hline
SERVICE & Normal & 1 \\ \hline
SETTINGS\_INAPP\_NOTI & Normal & 1 \\ \hline
STORAGE & Normal & 1 \\ \hline
SUBSCRIBED\_FEEDS\_READ & Normal & 1 \\ \hline
SYNC & Normal & 1 \\ \hline
SYSTEM\_UI\_VISIBILITY\_EXTENSION & Normal & 1 \\ \hline
TYPE\_APPLICATION\_OVERLAY & Normal & 1 \\ \hline
UPDATE & Normal & 1 \\ \hline
UPDATE\_BADGE & Normal & 1 \\ \hline
UPDATE\_EXISTS & Normal & 1 \\ \hline
VPN & Normal & 1 \\ \hline
WRITE\_ALARM & Normal & 1 \\ \hline
WRITE\_GSERVICES & Normal & 1 \\ \hline
WRITE\_History & Normal & 1 \\ \hline
WRITE\_SM\_DATA & Normal & 1 \\ \hline
camera & Normal & 1 \\ \hline
data & Normal & 1 \\ \hline
i18n\_security & Normal & 1 \\ \hline
i18n\_security\_lite & Normal & 1 \\ \hline
keeplive & Normal & 1 \\ \hline
ownreceiver & Normal & 1 \\ \hline
self & Normal & 1 \\ \hline
TOKEN\_62335eae576a847248.. & Normal & 0 \\ \hline
\end{longtable}}
